# Supplementary material for: WikiContradict: A Benchmark for Evaluating LLMs on Real-World Knowledge Conflicts from Wikipedia
Source: arXiv:2406.13805 source file (2024-06-19)
Supplement: Supplementary file 1 [file Appendix_B_Additional_Human_Evaluation.pdf]

# Prompt 5.1-5.4

## Prompt 5.1

Provide a short answer for the following question based on the given context. Carefully investigate the given context and provide a concise response that reflects the comprehensive view of the context, even if the answer contains contradictory information reflecting the heterogeneous nature of the context.

Question: {Question}
Context: {Passage 2} + {Passage 1}

## Prompt 5.2

Context: {Passage 1} + {Passage 2}

Does the above provided context contain conflicting information that could result in different answers to the question {Question}?" Provide a short answer followed by a concise explanation.

## Prompt 5.3

Provide a short answer for the following question based on the given context. Carefully investigate the given context and provide a concise response that reflects the comprehensive view of the context, even if the answer contains contradictory information reflecting the heterogeneous nature of the context.

Question: {Question}
Context: {Passage 1’} + {Passage 2’}

## Prompt 5.4

Context: {Passage 1’} + {Passage 2’}

Does the above provided context contain conflicting information that could result in different answers to the question {Question}?" Provide a short answer followed by a concise explanation.

# Additional Human Evaluation Results

| | Mistral-7b-instruct | | | Mixtral-8x7b-instruct | | | Llama-2-70b-chat | | | Llama-3-70b-instruct | | | GPT-4 | | |
|---|---|---|---|---|---|---|---|---|---|---|---|---|---|---|---|
| **Prompt Template 5.1** | | | | | | | | | | | | | | | |
| correct | 22.9 | 30.0 | 11.8 | 14.6 | 16.7 | 5.9 | 17.0 | 27.6 | 0.0 | 54.2 | 70.0 | 23.5 | 12.5 | 16.7 | 5.9 |
| partially correct | 72.9 | 66.7 | 82.4 | 70.8 | 73.3 | 70.6 | 80.9 | 72.4 | 94.1 | 45.8 | 30.0 | 76.5 | 81.3 | 83.3 | 76.5 |
| incorrect | 4.2 | 3.3 | 5.9 | 14.6 | 10.0 | 23.5 | 2.1 | 0.0 | 5.9 | 0.0 | 0.0 | 0.0 | 6.3 | 0.0 | 17.6 |
| **Prompt Template 5.2** | | | | | | | | | | | | | | | |
| correct | 35.4 | 40.0 | 29.4 | 4.2 | 6.7 | 0.0 | 76.6 | 89.7 | 52.9 | 77.1 | 93.3 | 47.1 | 89.6 | 96.7 | 76.5 |
| partially correct | 14.6 | 20.0 | 0.0 | 6.3 | 6.7 | 5.9 | 17.0 | 10.3 | 29.4 | 6.3 | 3.3 | 11.8 | 2.1 | 3.3 | 0.0 |
| incorrect | 50.0 | 40.0 | 70.6 | 72.9 | 76.7 | 70.6 | 6.4 | 0.0 | 17.6 | 14.6 | 3.3 | 35.3 | 8.3 | 0.0 | 23.5 |
| **Prompt Template 5.3** | | | | | | | | | | | | | | | |
| correct | 87.5 | 93.3 | 82.4 | 85.4 | 83.3 | 88.2 | 87.2 | 96.6 | 76.5 | 89.6 | 96.7 | 82.4 | 87.5 | 96.7 | 70.6 |
| partially correct | 6.3 | 3.3 | 5.9 | 4.2 | 6.7 | 0.0 | 2.1 | 0.0 | 5.9 | 2.1 | 0.0 | 5.9 | 2.1 | 0.0 | 5.9 |
| incorrect | 6.3 | 3.3 | 11.8 | 10.4 | 10.0 | 11.8 | 10.6 | 3.4 | 17.6 | 8.3 | 3.3 | 11.8 | 10.4 | 3.3 | 23.5 |
| **Prompt Template 5.4** | | | | | | | | | | | | | | | |
| correct | 66.7 | 70.0 | 64.7 | 83.3 | 83.3 | 82.4 | 12.8 | 6.9 | 23.5 | 47.9 | 50.0 | 41.2 | 43.8 | 50.0 | 35.3 |
| partially correct | 4.2 | 6.7 | 0.0 | 2.1 | 3.3 | 0.0 | 23.4 | 24.1 | 17.6 | 4.2 | 3.3 | 5.9 | 14.6 | 10.0 | 23.5 |
| incorrect | 29.2 | 23.3 | 35.3 | 2.1 | 3.3 | 0.0 | 63.8 | 69.0 | 58.8 | 45.8 | 43.3 | 52.9 | 41.7 | 40.0 | 41.2 |
