# Supplementary material for: WikiContradict: A Benchmark for Evaluating LLMs on Real-World Knowledge Conflicts from Wikipedia
Source: arXiv:2406.13805 source file (2024-06-19)
Supplement: Supplementary file 2 [file Appendix_C_LLM_Judge_Prompt.pdf]

# System prompt:

Please evaluate the response to a question under relaxed evaluation, where hallucinations, outdated information are allowed, as long as the primary answer is accurate.  Each response is evaluated as correct, partially correct, or incorrect. correct means the response accurately matches with all the answers in the correct answer list and it can contain contradictory answers that reflect the heterogeneous nature of the context, or the response aggregates the different answers and indicates that each answer is possible. In addition, the correct response should not indicate a preference for one answer over another. And the correct response should not combine two different correct answers without indicating the contradictory nature of these answers. partially correct means the response only matches with one of the answers in the correct answer list; or the response matches with all the answers in the correct answer list but it indicates a preference for one answer over another; or the response matches with all the answers in the correct answer list but it contains additional answers that doesn't match with any of the correct answers. incorrect means the response does not match with any of the correct answers in the correct answer list, or the response merely combines two contradictory answers from the correct answer list and indicates that both of them are possible. Note that for each question, there are multiple correct answers based on different sources even though these correct answers contradict each other. Please credit the response only if it provides a list of confident and definitive answers that match with the answers in the correct answer list, or the correct answers can be obviously inferred from the response. The primary or final answers when standing alone must be accurate. Any additional information that is provided must not contradict the primary answers or reshape one's perception of them. For answers that involve names of entities (e.g., people), complete names or commonly recognized names are expected. Regarding numerical answers, approximate numbers are generally not accepted unless explicitly included in the ground-truth answers. We accept responses that contain hallucinated or outdated information that does not significantly impact the primary answers.

# Examples

### Example 1

question: How old is the world's oldest verified living person?

correct_answers: 115 years old | 117 years old

response: As of today the most up-to-date and relevant information regarding this query is as follows. The oldest verified living person is Maria Branyas Morera, who was born on March 4, 1907, making her 117 years old.

comment: The primary answer in the response (117 years old) is partially correct as it only matched with with one of the correct answers (117 years old) and it doesn't mention another answer (115 years old). Thus, the response is partially correct.

evaluation: partially correct

### Example 2

question: How old is the world's oldest verified living person?

correct_answers: 115 years old | 117 years old

response: According to the context, the oldest verified living person is Maria Branyas Morera, who is both 115 years old and 117 years old.

comment: Although the primary answer contains all correct answers (115 years old and 117 years old) that matches with the correct answers, it is logically incorrect because a person cannot have two ages at the same time. Thus, the response is incorrect.

evaluation: incorrect

### Example 3

question: How old is the world's oldest verified living person?,

correct_answers: 115 years old | 117 years old

response: According to the context, one source claims that the oldest verified living person is Maria Branyas Morera, who is 117 years old. However, another source claims that she is 115 years old.

comment: The answer contains all correct answers: 115 years old and 117 years old, and it points out that these two answers are from different sources, which is logically possible. Thus, the response is correct.

evaluation: correct

## Example 4

question: How old is the world's oldest verified living person?,

correct_answers: 115 years old | 117 years old

response: According to the context, the oldest verified living person is Maria Branyas Morera, who is either 117 years old or 115 years old.

comment: The answer contains all correct answers: 115 years old and 117 years old that aggregates the different answers from different sources, which is logically possible. Thus, the response is correct.

evaluation: correct

## Example 5

question: How many books has Colleen Hoover published in 2020?

correct_answers: 26 books | 27

response: according to some sources, Colleen Hoover has published 26 books in 2020. However, other sources claim that it has published 27 books in 2020.

comment: The response accurately provides two answers (26 books and 27 books) based on different sources. It recognized the two sources that provide different answers. These two answers match with all correct answers (26 books, 27). Thus, the response is correct.

evaluation: correct

## Example 6

question: How many books has Colleen Hoover published in 2020?

correct_answers: 26 books | 27

response: Colleen Hoover has published 26 books in 2020.

comment: The response only provides one answers (26 books) based on the given context, which matched with one of the answers in the correct answer list. Thus, the response is particially correct.

evaluation: partically correct

## Example 7

question: How many member nations exist in the United Nations?

correct_answers: 193 members | 194 member states

response: As of my last update in April 2023, there were 191 member nations in the United Nations. Please note that this information may have changed since then, so it is advisable to check the latest information from the United Nations or other reliable sources.

comment: The primary answer in the response (191 member nations) does not match with any of the correct answers (193 member states or 194 members). Thus, the response is incorrect.

evaluation: incorrect

## Example 8

question: How many member nations exist in the United Nations?

correct_answers: 193 members | 194 member states

response: Although some sources claim that there are 193 member nations in the United Nations, the UN is made up of 194 member states.

comment: Althought the primary answer mentions two answers (193 members, 104 member states) that match with the correct answers, the response indicates a preference of one answer (194 member states) over the other (193 members). Thus, the response is partically correct.

evaluation: partically correct

# Testing instance

question: {Question}

correct_answers: {Answer1} | {Answer2}

response: {LLM response}

comment:
