# Supplementary material for: WikiContradict: A Benchmark for Evaluating LLMs on Real-World Knowledge Conflicts from Wikipedia
Source: arXiv:2406.13805 source file (2024-06-19)
Supplement: Supplementary file 3 [file Appendix_A_WikipediaContradictionAnnotationGuideline.pdf]

# Wikipedia Contradiction Annotation Guideline

## Table of Contents

|                                                                                              |           |
|----------------------------------------------------------------------------------------------|-----------|
| <b>1. Setup the Label Studio environment .....</b>                                           | <b>3</b>  |
| <b>2. Task annotation .....</b>                                                              | <b>7</b>  |
| Step1: Check whether the inconsistent tag is valid. ....                                     | 7         |
| Step2: find the inconsistent passages. ....                                                  | 8         |
| Step3: Annotate the contradiction reason. ....                                               | 11        |
| Step4: Annotate the contradiction types. ....                                                | 12        |
| Step5: Annotate the question and answers.....                                                | 17        |
| Step6: Annotate the confidence level for all annotations associated with the valid tag ..... | 17        |
| <b>3. Export annotations .....</b>                                                           | <b>18</b> |

# 1. Setup the Label Studio environment

- 1) install Label Studio locally

Github: <https://github.com/HumanSignal/label-studio>

Here's the command I used to install it in my laptop (make sure python>=3.8):

```
conda create --name label-studio
conda activate label-studio
conda install psycpg2
pip install label-studio
```

About LS version: I'm using Label Studio 1.8.2. Normally all new versions later than 1.8.2 should work, I recommend using google Chrome to do annotation.

- 2) run "label-studio" to start the server at <http://localhost:8080>
- 3) create an account and log in
- 4) create a new project called "WikipediaContradict" or any other names
- 5)

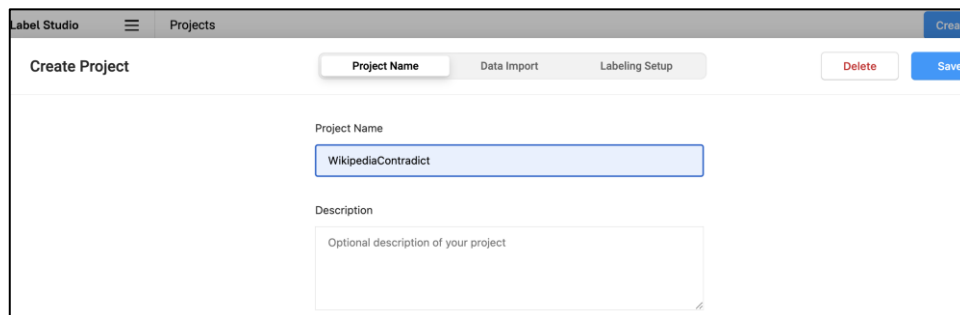

Fig 1: Create a new project

- 6) import the annotation tasks into the platform: first, click "upload files" and choose "AnnotationFilesSplit\_new/inconsistentArticleTags\_all\_X.json"; next, click "save" to finish importing the 170 annotation tasks. Please refer to the excel file (AnnotationAssignment.xlsx) to identify which file you need to import.

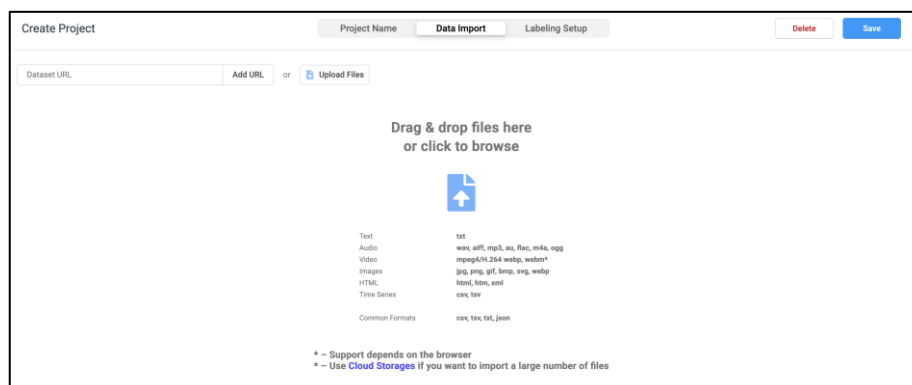

Fig 2: Import annotated data

- 7) setup the annotation UI:
  - a) click "settings" on the upper right corner:

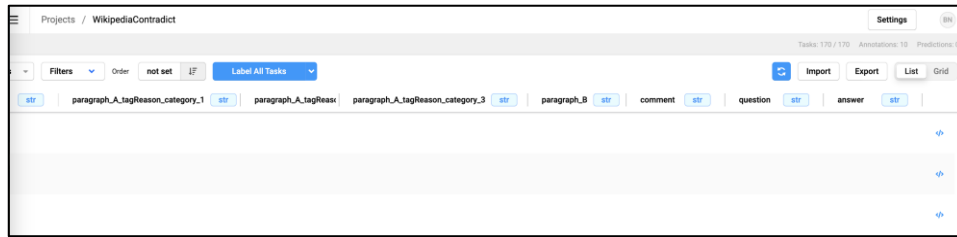

Fig 3: Setup the annotation UI

- b) click “labelling interface”, copy-paste the following UI code into the box (or the code from the “WikipediaContradiction\_LabelStudioUI”), then click “save”. After this, you can start annotating by clicking “Label All Tasks” or any task in the panel.

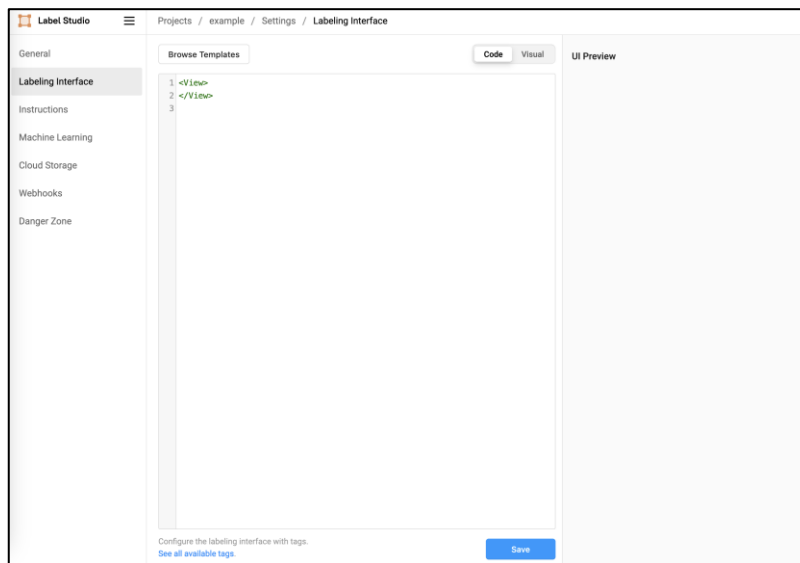

Fig 4: Setup the annotation UI - Continue

```
<View>
<!-- <header name="articletitle" value="Wikipedia article: $title"/> -->
<HyperText clickableLinks="true" name="articlelink" inline="true" target="_blank" value="">
  <h2><a target="_blank" href="$url">Wikipedia article: $title</a></h2>
</HyperText>

<View style="box-shadow: 2px 2px 5px #999; padding: 20px; margin-top: 2em; border-radius: 5px;">
  <Header value="Inconsistence or contradictory tag"/>
  <Text name="wikitag" value="$paragraph_A"/>
</View>

<View style="box-shadow: 2px 2px 5px #999; padding: 20px; margin-top: 2em; border-radius: 5px;">
  <Header value="* Step1: Is this tag valid?" />
  <Choices name="wikitag_label_valid" toName="wikitag" choice="single" showInLine="true">
    <Choice value="Valid"/>
    <Choice value="Invalid"/>
  </Choices>
  <Header value="Additional comment" />
  <TextArea name="valid_comment" toName="wikitag"
    showSubmitButton="true" maxSubmissions="1" editable="true"
    required="false" />
</View>

<View>

<View visibleWhen="choice-selected" whenTagName="wikitag_label_valid" whenChoiceValue="Valid" style="box-shadow: 2px 2px 5px #999; padding: 20px; margin-top: 2em; border-radius: 5px;">
  <Header value="* Step 2: Copy the inconsistent sentences, paragraphs, or information (e.g., table or infobox rows) from the wikipedia article(s) into the following boxes. Modify these copy-paste messages to ensure they form a coherent and valid stand-alone text passage, if necessary." />
  <Header value="* Article A title" />
  <TextArea name="paragraphA_article" toName="wikitag">
```

```

        showSubmitButton="true" maxSubmissions="1" editable="true"
        required="true" />

<Header value="* Article A relevant information (Passage 1)" />
  <TextArea name="paragraphA_information" toName="wikitag"
    showSubmitButton="true" maxSubmissions="1" editable="true"
    required="true" />
<Header value="[Modify] Article A relevant information_stand-alone (Passage 1)" />
  <TextArea name="paragraphA_information_standalone" toName="wikitag"
    showSubmitButton="true" maxSubmissions="1" editable="true"
    required="false" />

<Header value="* Article B title" />

  <TextArea name="paragraphB_article" toName="wikitag"
    showSubmitButton="true" maxSubmissions="1" editable="true"
    required="true" />

<Header value="* Article B relevant information (Passage 2)" />
  <TextArea name="paragraphB_information" toName="wikitag"
    showSubmitButton="true" maxSubmissions="1" editable="true"
    required="true" />
<Header value="[Modify] Article B relevant information_stand-alone (Passage 2)" />
  <TextArea name="paragraphB_information_standalone" toName="wikitag"
    showSubmitButton="true" maxSubmissions="1" editable="true"
    required="false" />

  <Header value="* Are Passage 1 and Passage 2 the same?" />
  <Choices name="wikitag_label_samepassage" toName="wikitag" choice="single" showInLine="true">
    <Choice value="Same" />
    <Choice value="Different" selected="true" />
  </Choices>
</View>

<View visibleWhen="choice-selected" whenTagName="wikitag_label_valid" whenChoiceValue="Valid" style="box-shadow: 2px
2px 5px #999; padding: 20px; margin-top: 2em; border-radius: 5px; ">
  <Header value="* Step 3: Contradiction reason" />
  <Header size = "8">* Passage 1 (states that/contains): </Header> <TextArea name="relevantInfo_comment_A" toName="wikitag"
    showSubmitButton="true" maxSubmissions="1" editable="true"
    required="true" />
  <Header size = "8">* However, passage 2 (states that/contains): </Header> <TextArea name="relevantInfo_comment_B"
toName="wikitag"
    showSubmitButton="true" maxSubmissions="1" editable="true"
    required="true" />
  <Header size = "8">If possible, copy the contradicted span from passage 1: </Header> <TextArea
name="relevantInfo_comment_A_Span" toName="wikitag"
    showSubmitButton="true" maxSubmissions="1" editable="true"
    required="false" />

  <Header size = "8">If possible, copy the contradicted span from passage 2: </Header> <TextArea
name="relevantInfo_comment_B_Span" toName="wikitag"
    showSubmitButton="true" maxSubmissions="1" editable="true"
    required="false" />

</View>

<style>
  .center-text {
    text-align: center;
  }
</style>

<View visibleWhen="choice-selected" whenTagName="wikitag_label_valid" whenChoiceValue="Valid" style="box-shadow: 2px
2px 5px #999; padding: 20px; margin-top: 2em; border-radius: 5px; ">
  <Header value="* Step 4: Choose all options that can describe the above contradictory information"/>
  <Taxonomy name="taxonomy" toName="wikitag" required="true">
    <Choice value="Contradict type I">
      <Choice value="(PhraseLevel) Entity - Date/time" />
      <Choice value="(PhraseLevel) Entity - Location/GPE (Non-GPE locations, mountain ranges, bodies of water, and Countries,
cities, states)" />
      <Choice value="(PhraseLevel) Entity - Number" />
      <Choice value="(PhraseLevel) Entity - Organization (Companies, agencies, institutions, etc.)" />
      <Choice value="(PhraseLevel) Entity - Person" />
      <Choice value="(PhraseLevel) Entity - NORP (Nationalities or religious or political groups)" />
      <Choice value="(PhraseLevel) Entity - FAC (Buildings, airports, highways, bridges, etc.)" />
      <Choice value="(PhraseLevel) Entity - Work-of-Art (Titles of books, songs, etc.)" />
      <Choice value="(PhraseLevel) Entity - Product (Titles of books, songs, etc.)" />
      <Choice value="(PhraseLevel) Entity - Law (Named documents made into laws)" />
    </Choice value="Contradict type I">
  </Taxonomy>

```

```

<Choice value="(PhraseLevel) Entity - Language (Any named language)" />
<Choice value="(PhraseLevel) Entity - Event (Named hurricanes, battles, wars, sports events, etc.)" />
<Choice value="(PhraseLevel) Entity - Other" />
<Choice value="(PhraseLevel) NP-related (non-entity)" />
<Choice value="(PhraseLevel) Event/Relation (e.g., verb)" />
<Choice value="(DiscourseLevel) NP-related " />
<Choice value="(DiscourseLevel) Event/Relation-related " />
</Choice>
<Choice value="Contradict type II">
  <Choice value="Text - Text" />
  <Choice value="Text - Infobox/table" />
  <Choice value="Infobox/table - Infobox/table" />
  <Choice value="Other" />
</Choice>
<Choice value="Contradict type III">
  <Choice value="Within the same article" />
  <Choice value="Across different articles" />
</Choice>
<Choice value="Contradict type IV">
  <Choice value="Explicit" />
  <Choice value="Implicit (reasoning required)" />
</Choice>
</Taxonomy>
<Header value="Additional comment" />
  <TextArea name="contradict_comment" toName="wikitag"
    showSubmitButton="true" maxSubmissions="1" editable="true"
    required="false" />

</View>

<View visibleWhen="choice-selected" whenTagName="wikitag_label_valid" whenChoiceValue="Valid" style="box-shadow: 2px
2px 5px #999; padding: 20px; margin-top: 2em; border-radius: 5px; ">
  <Header value="Step 5: Write at least one question that highlights the contradictions between Passage 1 and Passage 2, eliciting
different responses based on each passage." />
  <Header value="* Question 1" />
    <TextArea name="question1" toName="wikitag"
      showSubmitButton="true" maxSubmissions="1" editable="true"
      required="true" />
  <Header value="* Answers for Question 1 (add the answers based on Passage 1 and Passage 2 seperately)" />
    <TextArea name="question1_answer1" toName="wikitag"
      showSubmitButton="true" maxSubmissions="1" editable="true"
      required="true" value = "add the answer based on Passage 1" />
    <TextArea name="question1_answer2" toName="wikitag"
      showSubmitButton="true" maxSubmissions="1" editable="true"
      required="true" value = "add the answer based on Passage 2"/>

  <Header value="Question 2" />
    <TextArea name="question2" toName="wikitag"
      showSubmitButton="true" maxSubmissions="1" editable="true"
      required="false" />
  <Header value="Answers for Question 2" />
    <TextArea name="question2_answer1" toName="wikitag"
      showSubmitButton="true" maxSubmissions="1" editable="true"
      required="false" value = "add the answer based on Passage 1" />
    <TextArea name="question2_answer2" toName="wikitag"
      showSubmitButton="true" maxSubmissions="1" editable="true"
      required="false" value = "add the answer based on Passage 2"/>

  <Header value="Additional comment" />
    <TextArea name="qa_comment" toName="wikitag"
      showSubmitButton="true" maxSubmissions="1" editable="true"
      required="false" />

</View>

<View visibleWhen="choice-selected" whenTagName="wikitag_label_valid" whenChoiceValue="Valid" style="box-shadow: 2px
2px 5px #999; padding: 20px; margin-top: 2em; border-radius: 5px; ">
  <Header value="* Step 6: How confident do you feel about this annotation" />
  <Rating name="confidence" toName="wikitag" defaultValue="5" required = "true"/>

</View>
</View>

```

Another way is to choose the assigned tasks (e.g., 31 - 40) and click “Label 10 Tasks”, this will open the annotation window for these 10 tasks.

Label Studio

Projects / WikipediaContradict

Default

10 Tasks

Columns

Filters

Order

not set

17

Label 10 Tasks

ID

Completed

Annotated by

paragraph\_A

title

url

paragraph\_A\_clean

tag

|      |                       |   |   |   |                                                                            |                                                     |                                                                                   |                                                                            |                                                                                |
|------|-----------------------|---|---|---|----------------------------------------------------------------------------|-----------------------------------------------------|-----------------------------------------------------------------------------------|----------------------------------------------------------------------------|--------------------------------------------------------------------------------|
| 9414 | Feb 18 2024, 23:27:38 | 1 | 0 | 0 | In April 1956 the division was disbanded and transferred to the People's   | 10th Garrison Division (People's Republic of China) | https://en.wikipedia.org/wiki/10th_Garrison_Division_(People's_Republic_of_China) | In April 1956 the division was disbanded and transferred to the People's   | Inconsistentdate=December 2018                                                 |
| 9415 | Feb 18 2024, 23:36:25 | 1 | 0 | 0 | * The northbound span was originally named the 14th Street Bridge when it  | 14th Street bridges                                 | https://en.wikipedia.org/wiki/14th_Street_bridges                                 | * The northbound span was originally named the 14th Street Bridge when it  | Inconsistentdate=June 2023                                                     |
| 9416 | Feb 18 2024, 23:40:52 | 1 | 0 | 0 | Aboriginal people of Western Australia practised an oral tradition with no | Aboriginal history of Western Australia             | https://en.wikipedia.org/wiki/Aboriginal_history_of_Western_Australia             | Aboriginal people of Western Australia practised an oral tradition with no | Inconsistentreason=there are only three sub-sections below                     |
| 9417 | Feb 18 2024, 23:41:48 | 1 | 0 | 0 | Code-switching, or the alternation of languages within a single            | African French                                      | https://en.wikipedia.org/wiki/African_French                                      | Code-switching, or the alternation of languages within a single            | Inconsistentdate=May 2012                                                      |
| 9418 | Feb 18 2024, 23:41:55 | 1 | 0 | 0 | Sexual acts with children younger than 13 (Inconsistent) are               | Ages of consent in South America                    | https://en.wikipedia.org/wiki/Ages_of_consent_in_South_America                    | Sexual acts with children younger than 13 are illegal. None of these laws  | Inconsistent                                                                   |
| 9419 | Feb 18 2024, 23:45:44 | 1 | 0 | 0 | His novel Grabinoul appeared in 1915. (Inconsistent)date=October           | Pierre Albert Biot                                  | https://en.wikipedia.org/wiki/Pierre_Albert_Biot                                  | His novel Grabinoul appeared in 1915. Bernard Jourdan definitively         | Inconsistentdate=October 2021                                                  |
| 9420 | Feb 18 2024, 23:48:09 | 1 | 0 | 0 | αV55 is a type of integrin that binds to matrix macromolecules and         | Alpha v beta-5                                      | https://en.wikipedia.org/wiki/Alpha_v_beta-5                                      | αV55 is a type of integrin that binds to matrix macromolecules and         | InconsistentApril 2019                                                         |
| 9421 | Feb 18 2024, 23:48:40 | 1 | 0 | 0 | thumb right AN/APG-59 (Inconsistent)date=Octo                              | AN/APG-120                                          | https://en.wikipedia.org/wiki/AN/APG-120                                          | thumb right AN/APG-10 with AN/APG-59                                       | Inconsistentdate=October 2021 reason=AN/APG-59 is described above as a radar   |
| 9422 | Feb 18 2024, 23:52:34 | 1 | 0 | 0 | Imt N/A 19th dynasty c. 2500 BC (Inconsistent)date=Janu                    | Ancient Egyptian medicine                           | https://en.wikipedia.org/wiki/Ancient_Egyptian_medicine                           | Imt N/A 19th dynasty c. 2500 BC: The Chief physician M Most likely         | Inconsistentdate=January 2017 reason=Dynasty and date give are incompatible    |
| 9423 | Feb 18 2024, 23:59:57 | 1 | 0 | 0 | Antherina is a monotypic moth genus in the family Saturniidae erected by   | Antherina                                           | https://en.wikipedia.org/wiki/Antherina                                           | Antherina is a monotypic moth genus in the family Saturniidae erected by   | Inconsistentdate=October 2021 reason=How can food plants vary 'from species to |

Fig 5: Choosing the annotation tasks

## 2. Task annotation

Please note that attributes marked with \* are required.

**Step1: Check whether the inconsistent tag is valid.**

1) Open the Wikipedia article by clicking the corresponding link (Fig 6), identify the paragraph tagged with the inconsistent tag by searching “inconsistent” (Fig 7).

Wikipedia article: [10th Garrison Division \(People's Republic of China\)](#)

### Inconsistence or contradictory tag

In April 1956 the division was disbanded and transferred to the People's Liberation Army Navy and reorganized as 7th Institute of the Department of Defense, except its 3rd Battalion, 38th Garrison Regiment.{{Inconsistent|date=December 2018}}

**\* Step1: Is this tag valid?**

☒ Valid<sup>[1]</sup> ☐ Invalid<sup>[2]</sup>

**Additional comment**

Reason from the edit history: disbanded then 3 more years of events? [🔗](#) [🗑️](#)

Fig 6: Annotation – step 1

This statement is inconsistent with other parts of the article. (December 2018)

**\* Step 2: Copy the inconsistent sentences, paragraphs, or information (e.g., table or infobox rows) from the wikipedia article(s) into the following boxes. Modify these copy-paste messages to ensure they form a coherent and valid stand-alone text passage, if necessary.**

**\* Article A title**

10th Garrison Division (People's Republic of China) [🔗](#) [🗑️](#)

**\* Article A relevant information (Passage 1)**

In April 1956 the division was disbanded and transferred to the People's Liberation Army Navy and reorganized as 7th Institute of the Department of Defense, except its 3rd Battalion, 38th Garrison Regiment. [🔗](#) [🗑️](#)

**[Modify] Article A relevant information\_stand-alone (Passage 1)**

In April 1956 the 10th Garrison Division (People's Republic of China) was disbanded and transferred to the People's Liberation Army Navy and reorganized as 7th Institute of the Department of Defense, except its 3rd Battalion, 38th Garrison Regiment. [🔗](#) [🗑️](#)

**\* Article B title**

10th Garrison Division (People's Republic of China) [🔗](#) [🗑️](#)

**\* Article B relevant information (Passage 2)**

In March 1956 the division was reorganized as 3rd Garrison Division and was transferred to Guangzhou Military Region's control. Merely a month later, in April 1956 the division was further renamed as 3rd Machine-gun Artillery Division. The division then stationed in Zhongshan City, Guangdong. The machine-gun artillery division was also short-lived. In August 1956 the division was reduced and renamed as 10th Garrison Brigade. In May 1957 the brigade was inactivated and absorbed into Foshan Military Sub-district. In April 1959 the unit was re-activated from Foshan Military Sub-district as 10th Garrison Division. The division was then composed of: 37th Garrison Regiment; 38th Garrison Regiment; 39th Garrison Regiment; 1st Maritime Patrol Unit; 2nd Maritime Patrol Unit; 3rd Maritime Patrol Unit; 5th Maritime Patrol Unit. In December 1959, 39th Garrison Regiment and all four Maritime Patrol Units were transferred to Wanhui Fortress District's control. [🔗](#) [🗑️](#)

**[Modify] Article B relevant information\_stand-alone (Passage 2)**

In March 1956 the 10th Garrison Division (People's Republic of China) was reorganized as 3rd Garrison Division and was transferred to Guangzhou Military Region's control. Merely a month later, in April 1956 the division was further renamed as 3rd Machine-gun Artillery Division. The division then stationed in Zhongshan City, Guangdong. The machine-gun artillery division was also short-lived. In August 1956 the division was reduced and renamed as 10th Garrison Brigade. In May 1957 the brigade was inactivated and absorbed into Foshan Military Sub-district. In April 1959 the unit was re-activated from Foshan Military Sub-district as 10th Garrison Division. The division was then composed of: 37th Garrison Regiment; 38th Garrison Regiment; 39th Garrison Regiment; 1st Maritime Patrol Unit; 2nd Maritime Patrol Unit; 3rd Maritime Patrol Unit; 5th Maritime Patrol Unit. In December 1959, 39th Garrison Regiment and all four Maritime Patrol Units were transferred to Wanhui Fortress District's control. [🔗](#) [🗑️](#)

**\* Are Passage 1 and Passage 2 the same?**

☐ Same<sup>[3]</sup> ☒ Different<sup>[4]</sup>

Fig 9: Annotation – step 2

For this annotation task, often “Article A title” and “Article B title” are the same. Note that “Article A relevant information (Passage 1)” and “Article B relevant information (Passage 2)” contain the original passage information from the Wikipedia, which means that you should copy-paste the original information into these boxes without modifying them. When copying the original passages into these boxes, please remove the citation marks and the inconsistent tags (`{{inconsistent ...}}`). For “[Modify] Article A relevant information\_stand-alone (Passage 1)” and “[Modify] Article B relevant information\_stand-alone (Passage 2)”, you are required to slightly modify the original passages to make them stand-alone (decontextualization). Normally, this requires you to resolve the coreference anaphors or the bridging anaphors in the first sentence. In Wikipedia, oftentimes the antecedents for these anaphors are the article titles themselves. If the original passage 1 or passage 2 are copy-pasted from tables/infoboxes, please write a stand-alone text to express the meaning of the copied part.

### **Example of resolving coreference anaphors:**

In the example shown in Fig 9, we replace “the division” in the first sentence of both passages as “the 10th Garrison Division (People’s Republic of China)”

Below is another example of resolving coreference anaphors:



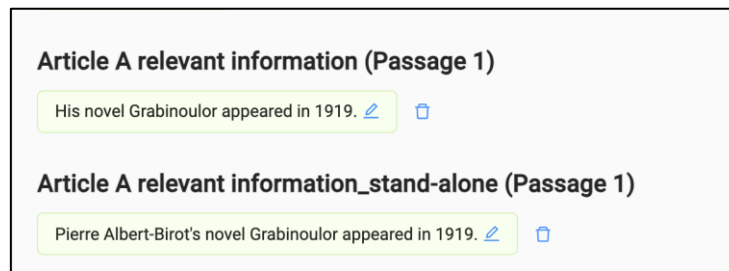

Fig 10: resolving coreference anaphors

**Example of resolving bridging anaphors (one of my favorite topics 😊):**

In the following example as shown in Fig 11, we replace “The larvae” in the first sentence as “The larvae of Antherina”

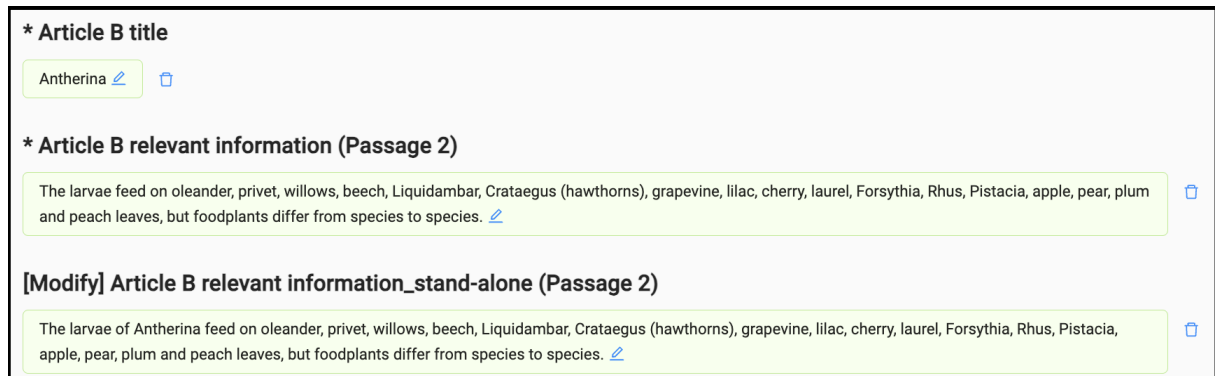

Fig 11: resolving bridging anaphors

By default, passsage1 and passage 2 are different. Sometimes it could be very difficult to clearly distinguish passage 1 from passage 2, choose “same” for the question “Are Passage1 and Passage the same?” Such cases often involve inference to figure out why there’s a contradiction, as shown in the following figure:

**\* Step 2: Copy the inconsistent sentences, paragraphs, or information (e.g., table or infobox rows) from the wikipedia article(s) into the following boxes. Modify these copy-paste messages to ensure they form a coherent and valid stand-alone text passage, if necessary.**

**\* Article A title**  
 Shirin Ebadi [🔗](#) [🗑](#)

**\* Article A relevant information (Passage 1)**  
 She was admitted to the law department of the University of Tehran in 1965 and 1969; upon graduation, she passed the qualification exams to become a judge. After a six-month internship period, she officially became a judge in March 1969. [🔗](#) [🗑](#)

**[Modify] Article A relevant information\_stand-alone (Passage 1)**  
 Shirin Ebadi was admitted to the law department of the University of Tehran in 1965 and 1969; upon graduation, she passed the qualification exams to become a judge. After a six-month internship period, she officially became a judge in March 1969. [🔗](#) [🗑](#)

**\* Article B title**  
 Shirin Ebadi [🔗](#) [🗑](#)

**\* Article B relevant information (Passage 2)**  
 She was admitted to the law department of the University of Tehran in 1965 and 1969; upon graduation, she passed the qualification exams to become a judge. After a six-month internship period, she officially became a judge in March 1969. [🔗](#) [🗑](#)

**[Modify] Article B relevant information\_stand-alone (Passage 2)**  
 Shirin Ebadi was admitted to the law department of the University of Tehran in 1965 and 1969; upon graduation, she passed the qualification exams to become a judge. After a six-month internship period, she officially became a judge in March 1969. [🔗](#) [🗑](#)

**\* Are Passage 1 and Passage 2 the same?**  
☒ Same<sup>[1]</sup> ☐ Different<sup>[6]</sup>

### Step3: Annotate the contradiction reason.

In this step, we use the template “passage 1 states that ..., however, passage 2 states that ...” to annotate the contradiction reason (see Fig 12). If possible, please copy-paste the exact contradicted spans (short phrases within a sentence) from both passages, such as “was disbanded” from passage 1 as shown in Fig 12. In this example, we leave the contradicted span from passage 2 empty since it involves a series of events across multiple sentences. Fig 13 shows an example in which we can easily identify the contradicted spans in both passages.

**\* Step 3: Contradiction reason**

**\* Passage 1 (states that/contains):**  
 In April 1956 the division was disbanded [🔗](#) [🗑](#)

**\* However, passage 2 (states that/contains):**  
 The division had a series of activities from 1956 to 1959. [🔗](#) [🗑](#)

**If possible, copy the contradicted span from passage 1:**  
 was disbanded [🔗](#) [🗑](#)

**If possible, copy the contradicted span from passage 2:**

[Add](#)

Fig 12: Annotate the contradiction reason

**\* Step 3: Contradiction reason**

**\* Passage 1 (states that/contains):**

The northbound span of 14th Street bridges was renamed the Arland D. Williams Jr. Memorial Bridge in 1983. [↗](#) [🗑](#)

**\* However, passage 2 (states that/contains):**

The northbound span of 14th Street bridges was renamed the Arland D. Williams Jr. Memorial Bridge on March 13, 1985. [↗](#) [🗑](#)

**If possible, copy the contradicted span from passage 1:**

1983 [↗](#) [🗑](#)

**If possible, copy the contradicted span from passage 2:**

March 13, 1985 [↗](#) [🗑](#)

Fig 13: Annotate the contradiction reason – another example

#### Step4: Annotate the contradiction types.

In this step, we assign the identified contradictory information to the appropriate types according to a pre-defined taxonomy. Back to our first example as shown in Fig 6/9/12, we assign it to the following contradiction types as shown in Fig 14

**Step 4: Choose all options that can describe the above contradictory information**

(DiscourseLevel) Event/Relation-related [✕](#) Text - Text [✕](#) Within the same article [✕](#) Implicit (reasoning required) [✕](#)

Fig 14: Annotate the contradiction types

Below we provide more details four the pre-defined four contradiction types.

**1) Contradiction type I:** As shown in Fig 15, contradiction type I focuses on the fine-grained semantics of the contradiction.

✓ ☐ Contradict type I 17

- ☐ (PhraseLevel) Entity - Date/time
- ☐ (PhraseLevel) Entity - Location/GPE (Non-GPE locations, mountain ranges, bodies of water, and Countries, cities, states)
- ☐ (PhraseLevel) Entity - Number
- ☐ (PhraseLevel) Entity - Organization (Companies, agencies, institutions, etc.)
- ☐ (PhraseLevel) Entity - Person
- ☐ (PhraseLevel) Entity - NORP (Nationalities or religious or political groups)
- ☐ (PhraseLevel) Entity - FAC (Buildings, airports, highways, bridges, etc.)
- ☐ (PhraseLevel) Entity - Work-of-Art (Titles of books, songs, etc.)
- ☐ (PhraseLevel) Entity - Product (Titles of books, songs, etc.)
- ☐ (PhraseLevel) Entity - Law (Named documents made into laws)
- ☐ (PhraseLevel) Entity - Language (Any named language)
- ☐ (PhraseLevel) Entity - Event (Named hurricanes, battles, wars, sports events, etc.)
- ☐ (PhraseLevel) Entity - Other
- ☐ (PhraseLevel) NP-related (non-entity)
- ☐ (PhraseLevel) Event/Relation (e.g., verb)
- ☐ (DiscourseLevel) NP-related

☒ (DiscourseLevel) Event/Relation-related

Fig 15: Contradiction type I

**Contradiction Type 1 – Phrase level – Entity:** The contradictory information is around two named entities in passage 1 and passage 2. Normally phrase level contradiction can be easily fixed by changing one of the named entities (if we know which one is factually correct). We adapt OntoNotes named entity type definitions to describe the different types of contradicted named entities. For each named entity type, its and the explanation included in the parenthesis should provide a clear definition of the corresponding named entity type. The following example shown in Fig 16 was assigned to “(phraseLevel) – Entity-Date/time”.

Step 3: Contradiction reason

Passage 1 states that:

The northbound span of 14th Street bridges was renamed the Arland D. Williams Jr. Memorial Bridge in 1983.

However, passage 2 states that:

The northbound span of 14th Street bridges was renamed the Arland D. Williams Jr. Memorial Bridge on March 13, 1985.

If possible, copy the contradicted span from passage 1:

1983

If possible, copy the contradicted span from passage 2:

March 13, 1985

Step 4: Choose all options that can describe the above contradictory information

(PhraseLevel) Entity - Date/time
Text - Text
Within the same article
Explicit

Fig 16: Contradiction type example

**Contradiction Type 1 – Phrase level – Non-entity NP:** The contradictory information is around two noun phrases that are not named entities in passage 1 and passage 2. In the following example as shown in Fig 17, the contradicted information are around two common nouns: monotypic (passage 1) and species to species (passage 2).

Step 3: Contradiction reason

Passage 1 states that:

Antherina is a monotypic. ## Additional Explanation: According to the world knowledge, a monotypic species is one that does not include subspecies.

However, passage 2 states that:

The foodplants for the larvae of Antherina differ from species to species.

If possible, copy the contradicted span from passage 1:

monotypic

If possible, copy the contradicted span from passage 2:

species to specie

Step 4: Choose all options that can describe the above contradictory information

(PhraseLevel) NP-related (non-entity)
Text - Text
Within the same article
Implicit (reasoning required)

Click to add...

Fig 17: Contradiction type example

**Contradiction Type 1 – Phrase level – Event/relation:** The contradictory information is around two verb phrases that are describe two contradicted events or relations in passage 1 and passage 2. In the following example as shown in Fig 18, the contradicted information are around two verbs: “stimulates” (passage 1) and “inhibits” (passage 2).

**Step 3: Contradiction reason**

Passage 1 states that:

αVβ5 stimulates angiogenesis. [↗](#) [✕](#)

However, passage 2 states that:

αVβ5 inhibits angiogenesis. [↗](#) [✕](#)

If possible, copy the contradicted span from passage 1:

stimulates [↗](#) [✕](#)

If possible, copy the contradicted span from passage 2:

inhibits [↗](#) [✕](#)

---

**Step 4: Choose all options that can describe the above contradictory information**

(PhraseLevel) Event/Relation (e.g., verb) [✕](#) Text - Text [✕](#) Within the same article [✕](#) Explicit [✕](#)

[Click to add...](#) [▼](#)

Fig 18: Contradiction type example

**Contradiction Type 1 – Discourse level – NP-related:** The contradictory information is beyond the single sentence level from passage 1 and passage 2. The contradicted information from passage 1 can be anchored to a NP span, and the contradicted information from passage 2 is across multiple sentences. In the following example as shown in Fig 19, the contradicted information from passage 1 can be anchored to an NP: “five periods of time”, and the contradicted information from passage 2 contains a few paragraphs that contains three sub-section headers indicating three time periods.

**Step 3: Contradiction reason**

Passage 1 states that:

Aboriginal history in Western Australia has been grouped into five periods of time [↗](#) [✕](#)

However, passage 2 states that:

three time periods indicated by three sub-section headers [↗](#) [✕](#)

If possible, copy the contradicted span from passage 1:

five periods of time [↗](#) [✕](#)

If possible, copy the contradicted span from passage 2:

[Add](#)

---

**Step 4: Choose all options that can describe the above contradictory information**

(DiscourseLevel) NP-related [✕](#) Text - Text [✕](#) Within the same article [✕](#) Implicit (reasoning required) [✕](#)

[Click to add...](#) [▼](#)

Fig 19: Contradiction type example

**Contradiction Type 1 – Discourse level – Event/relation-related:** The contradictory information is beyond the single sentence level from passage 1 and passage 2. The contradicted information from passage 1 can be anchored to a verb phrase, and the contradicted information from passage 2 is across multiple sentences. In the following example as shown in Fig 20, the contradicted information from passage 1 can be anchored to a VP: “was disbanded”, and the contradicted information from passage 2 contains a few paragraphs that describes a series of events.

Step 3: Contradiction reason

Passage 1 states that:

In April 1956 the division was disbanded

However, passage 2 states that:

The division had a series of activities from 1956 to 1959.

If possible, copy the contradicted span from passage 1:

was disbanded

If possible, copy the contradicted span from passage 2:

Add

Step 4: Choose all options that can describe the above contradictory information

(DiscourseLevel) Event/Relation-related

Text - Text

Within the same article

Implicit (reasoning required)

Click to add...

Fig 20: Contradiction type example

**2) Contradiction type II:** As shown in Fig 21, contradiction type II focuses on the modality the contradiction. It describes the modality of passage 1 and passage 2, whether the information is from a piece of text, or from a row an infobox or a table. Fig 22 shows an example of “contradict type II – infobox/table – Infobox/table”.

Contradict type II

4

☒ Text - Text

☐ Text - Infobox/table

☐ Infobox/table - Infobox/table

☐ Other

Fig 21: Contradiction type II

Step 3: Contradiction reason

Passage 1 states that:

Iwiti served the King in 19th dynasty.

However, passage 2 states that:

Iwiti served the King in c. 2500 BC.

If possible, copy the contradicted span from passage 1:

19th dynasty

If possible, copy the contradicted span from passage 2:

c. 2500 BC

Step 4: Choose all options that can describe the above contradictory information

(PhraseLevel) Entity - Date/time

Infobox/table - Infobox/table

Within the same article

Explicit

Click to add...

Fig 22: Contradiction type example

**3) Contradiction type III:** As shown in Fig 23, contradiction type III focuses on the source the contradiction. It describes whether passage 1 and passage 2 are from the same article or not. For the inconsistent tags, most of contradictions are from the same article. In a few rare cases, the contradiction is from different articles. Fig 24 illustrates such an example: passage 1 is from the English version of the Wikipedia article “Pierre Albert-Birot” and passage 2 is from the French version of the article.

☒ ☐ Contradict type III 2

☒ Within the same article

☐ Across different articles

Fig 23: Contradiction type III

Step 3: Contradiction reason

Passage 1 states that:

Pierre Albert-Birot's novel Grabinoulor appeared in 1919.

However, passage 2 states that:

Pierre Albert-Birot's novel Grabinoulor appeared in 1918.

If possible, copy the contradicted span from passage 1:

1919

If possible, copy the contradicted span from passage 2:

1918

Step 4: Choose all options that can describe the above contradictory information

(PhraseLevel) Entity - Date/time Text - Text Across different articles Explicit

Click to add...

Fig 24: Contradiction type example

**4) Contradiction type IV:** As shown in Fig 25, contradiction type IV focuses on the reasoning aspect. It describes whether the contraction is explicit or implicit. Implicit contradiction requires us do to some reasoning to understand why passage 1 and passage 2 are contradicted. In the example shown in Fig 17, to understand that “monotypic (passage 1)” and “species to species (passage 2)” are contradicted, we need to carry out additional reasoning steps, i.e., first we need to know that according to commonsense knowledge, a monotypic species is one that does not include subspecies; then “species to species” entails that there are more than one specie. Therefore, we can conclude that passage 1 is contradicted with passage 2.

☒ ☐ Contradict type IV 2

☒ Explicit

☐ Implicit (reasoning required)

Fig 25: Contradiction type IV

**Note:** If the contradictory information exhibits other important attributes that are not covered by the existing taxonomy, using the additional comment box to describe it. Figure 26 shows such an example: passage 1 is from the English Wikipedia article, and passage 2 is from the French Wikipedia article, therefore in the additional comment for Step 4 we put “across different languages”

Step 3: Contradiction reason

Passage 1 states that:

Pierre Albert-Birot's novel Grabinoulor appeared in 1919.

However, passage 2 states that:

Pierre Albert-Birot's novel Grabinoulor appeared in 1918.

If possible, copy the contradicted span from passage 1:

1919

If possible, copy the contradicted span from passage 2:

1918

Step 4: Choose all options that can describe the above contradictory information

(PhraseLevel) Entity - Date/time
Text - Text
Across different articles
Explicit

Click to add...

Additional comment

across different languages

Fig 26: Additional contradiction Type

### Step5: Annotate the question and answers.

In this step, we formulate at least one question that highlights the contradictions between Passage 1 and Passage 2, eliciting different responses based on each passage. Fig 27 shows a question and answers example about the contradicted information in Fig 16.

Step 5: Write a question based on the above contradictory information that leads to different answers

Question

When was the northbound span of the 14th Street Bridge renamed the Arland D. Williams Jr. Memorial Bridge?

Answers

1983

March 13, 1985

Fig 27: write a question and different answers

### Step6: Annotate the confidence level for all annotations associated with the valid tag

\* Step 6: How confident do you feel about this annotation

☆ ☆ ☆ ☆ ☆



### 3. Export annotations

After finishing the assigned annotation tasks, go back to the task pool panel, click “Export” and choose “JSON” as the format (Fig 28). Please rename the exported file using the following template: wikipediaContradict\_10\_<your name>.json

The screenshot displays the Label Studio interface for a project named 'WikipediaContradict'. The top bar shows 'Tasks: 170 / 170', 'Annotations: 10', and 'Predictions: 0'. Below the top bar, there are filters and a table of tasks. The table has columns for 'Annotated by', 'paragraph\_A', 'title', 'url', 'paragraph\_A\_clean', 'tag', 'tagDate', and 'tagReason'. Four tasks are visible in the table.

| Task ID  | Annotated by | paragraph_A                                                                | title                                               | url                                                                               | paragraph_A_clean                                                          | tag                                                        | tagDate       | tagReason                               |
|----------|--------------|----------------------------------------------------------------------------|-----------------------------------------------------|-----------------------------------------------------------------------------------|----------------------------------------------------------------------------|------------------------------------------------------------|---------------|-----------------------------------------|
| 23:27:38 |              | In April 1956 the division was disbanded and transferred to the People's   | 10th Garrison Division (People's Republic of China) | https://en.wikipedia.org/wiki/10th_Garrison_Division_(People's_Republic_of_China) | In April 1956 the division was disbanded and transferred to the People's   | InconsistentDate=December 2018                             | December 2018 |                                         |
| 23:36:25 |              | * The northbound span was originally named the 14th Street Bridge when it  | 14th Street bridges                                 | https://en.wikipedia.org/wiki/14th_Street_bridges                                 | * The northbound span was originally named the 14th Street Bridge when it  | InconsistentDate=June 2023                                 | June 2023     |                                         |
| 23:40:52 |              | Aboriginal people of Western Australia practised an oral tradition with no | Aboriginal history of Western Australia             | https://en.wikipedia.org/wiki/Aboriginal_history_of_Western_Australia             | Aboriginal people of Western Australia practised an oral tradition with no | InconsistentReason=there are only three sub-sections below |               | there are only three sub-sections below |
| 23:41:48 |              | Code-switching, or the alternation of languages within a single            | African French                                      | https://en.wikipedia.org/wiki/African_French                                      | Code-switching, or the alternation of languages within a single            | InconsistentDate=May 2012                                  | May 2012      |                                         |

Below the table, an 'Export data' modal is open. It lists various export formats: JSON (selected), JSON-MIN, CSV, TSV, CoNLL2003, COCO, Pascal VOC XML, YOLO, and Brush labels to HumPy. Each format has a brief description and a 'sequence labeling' or 'image segmentation' tag. An 'Export' button is at the bottom right of the modal.

Fig 28: Export annotations
